# Supplementary material for: Disorder-induced stabilization of the quantum Hall ferromagnet
Source: arXiv:1510.04448 source file (2015-10-15)
Supplement: Supplementary file 1 [file QHFstab_arxiv_PIOT_SM.pdf]

# Disorder-induced stabilization of the quantum Hall ferromagnet: SUPPLEMENTARY INFORMATION

This supplemental material is organized in three main sections. Section I discusses the experimental aspects of the resistive NMR technique, section II gives further details on our procedure to estimate the spin polarization of the system, and the last section gives additional elements on how the experimental phase diagram of the 2DEG around filling factor $\nu = 1$ is built.

## I. FREQUENCY-PULSED RESISTIVELY-DETECTED NMR

### A. Principle and experimental details

In the presence of a strong coupling between electronic and nuclear spins, nuclear magnetic resonance (NMR) can be used to probe the electronic spin polarization of the 2DEG. In a simplified mean field view of the hyperfine coupling, polarized electrons create a local magnetic field $B_e$ coupling to the nuclear spins. This field reduces the Larmor resonance frequency of the nuclei by a quantity $K_S \propto nP$, the so-called Knight shift, proportional to the local electron density $n$ and electronic spin polarization $P$. In 2D systems containing a few nuclear spins, conventional (inductive) NMR lacks sensitivity, and alternative techniques have to be employed.[1–3] Among these techniques, Resistively-detected NMR (RDNMR)[3] is particulary well-suited for the study of a single 2DEG at very low temperatures. It relies on the dependence of the longitudinal resistance $R_{xx}$ of the 2DEG on the Zeeman energy gap, which can be written as $\Delta E_Z = g^* \mu_B (B + B_N)$, where $B_N$ is the effective nuclear magnetic field seen by the electron system (Overhauser field). At the NMR frequency, nuclear spins are depolarized and the amplitude of $B_N$ reduced, which affects the Zeeman gap and can therefore be detected as a variation in the longitudinal resistance $R_{xx}$. In some cases though, $R_{xx}$ is not sensitive to a change in the Zeeman energy, and this is typically the case in the close vicinity of $\nu = 1$ where $R_{xx}$ vanishes and the application of standard RDNMR is impossible. To overcome this limitation, pulsed-RDNMR schemes have been developed.[4,5] In this work we have used the frequency-pulsed Resistively-detected NMR that we have presented in Ref.5. The 2DEG is excited with a given frequency at the filling factor $\nu$ of interest for a certain time, and then switched back to a "sensitive" $R_{xx}$ detection point by the application of a gate voltage. The change in $R_{xx}$ is probed at the detection point with a frequency set to an off-resonant value (typically the initial starting frequency) to avoid any further excitation of the nuclear system while maintaining stable thermal conditions. The sequence is repeated at different excitation radio frequencies to reconstruct the NMR spectra. In the present case, we have generally used schemes with 4s excitation and 1s detection phases. Slow sweeps (typically 100 Hz steps giving a 20Hz/s rate) were used to approach a quasi-static response of the system, giving a more accurate estimation of the Knight shift.

The NMR response has been probed at fixed magnetic fields for different filling factors $\nu$ in the $\nu = 0.8 - 1.2$ range. A large amount of scans were recorded to increase our resolution up to about 0.001 in filling factor, in order to be able to resolve sharp changes in the polarization as a function of $\nu$. The basic density/ filling factor calibrations were first obtained by using the low magnetic field Hall voltage, but were fine-tuned by using the position of the integer/fractional QH states at mK temperature to enhance our precision on the filling factor determination in the $\nu = 1$ vicinity. Series of experiment were repeated for different magnetic fields, from 5T to 14T. The radio-frequency power range was varied between -5 dBm and +10 dBm to reach similar signals and bath conditions in the very different frequency range applied throughout the experiments. The electronic temperature was systematically determined from the resistance of the sample and its calibrated temperature dependence, and for the reported spectra is in the range 180-250 mK. These values were mainly limited by the electrical current injected in the 2DEG, typically about 50 nA. Such currents were necessary to keep a sufficient signal-to-noise-ratio to study the weak response in the close vicinity of $\nu = 1$.

### B. Lineshape and Knight shift

In the case of GaAs-2DEGs, the NMR frequency shift $\Delta f$ is given by:

$$\Delta f = \mathcal{A} P(n/W) \tag{1}$$

where $\mathcal{A}$ is the hyperfine coupling constant in the host material, $P$ the spin polarization of the system, $n$ the electron density and $W$ the spatial "thickness" of the (quasi-)2DEG. The $\mathcal{A}(n/W)$ term stands here for the local electronic density at the nuclear site. In real experimental systems, the NMR response can be broadened by various effects, and in particular by the profile of the electronic density (wave function) along the confinement axis (z) of the quasi-2D system.[4,6] In the case of pulsed-RDNMR, the use of excitation and detection points corresponding to significantly different electron densities (and potentially different wave function z-profile) can also give further modulation to the line shape, as shown in Ref.4.

In the present experiments, however, the RDNMR lineshapes could generally be well-reproduced by simply applying a broadening to the intrinsic shift described by Eq.1. These simulations are reported as solid lines in figure 1 in the main text. For the higher magnetic fields (9, 11 and 14T), the larger Knight shift enables us to see that the RDNMR response is rather symmetric around the $R_{xx}$ minimum and that no "low Knight shift tail" characteristic of a "peaked" electron distribution along z is observed. This suggests that the wave function in our system is rather smoothly varying along the confinement axis, meaning that Eq.1 is applicable and that the $R_{xx}$ minimum gives a good estimate of the resonance frequency position. This is also made possible thanks to the proximity of our excitation and detection points in the f-PRDNMR scheme used, which can be described by similar electronic wave functions.

We mention that the signals observed at high magnetic fields are quite unique in the sense that they display two well-separated features, a low frequency minimum, and a maximum close to $f_0$, with a nearly flat part in between. This observation, qualitively different from the usual dispersive lineshapes observed around (but further from) $\nu = 1$,[7] is made possible by the high degree of spin polarization and the high electron densities both producing a large Knight shift. It confirms our approach in which the RDNMR signal is made of the response of two independent electronic sub-systems.[8]

We stress that while the exact z-axis profile of the wave function does not need to be incorporated to reproduce most of the observed lineshapes, its total "width" remain important in defining the Knight shift, as seen in Eq.1 (see also section II.A). We have checked that even in the case of a $|\Psi^2| \sim cos(z)^2$ wave function profile, density-induced variations of $W$ in our experimental range ($\nu = 0.8 - 1.2$) shifted the NMR minimum within 2 percent of the expectations given by Eq.1. This ensures that the $R_{xx}$ minimum remains a good reference point to estimate the Knight shift in our limited filling factor range for excitation, detection, and calibration.

We finally mention that the choice to perform the present study on $^{71}Ga$ NMR, rather than the more generally used $^{75}As$ was motivated by different reasons. First, the smaller quadrupolar splitting in $^{71}Ga$ (typically 13 kHz) basically broadens the RDNMR minimum, rather than giving a potentially complex interplay with the max feature as observed in some cases for $^{75}As$ where the quadrupolar splitting is the order of (or larger than) the Knight shift[9]. This prevents apparent shifts of the minimum/maximum position, and allows for a double-check of the "$P = 0$ response" which can be inferred from the RDNMR maximum (high frequency response). Secondly, the slightly higher Knight shifts (see Ref.7) help to separate the minimum and maximum response in the lineshape, and limit possible overlap effects between the two responses when the spin polarization is low (we note that below a certain value of $P$ or electron density $n$, these effects shall be taken into account). We note that the choice of $^{71}Ga$ is nevertheless made at the expense of smaller signals due to the lower isotopic abundance.

## II. POLARISATION OF THE $\nu = 1$ STATE

### A. Calibration procedure

To be able to study the $\nu = 1$ QHF spin polarization in an absolute way, a Knight shift reference for a fully spin polarized state ($P = 1$) is required. As shown in previous measurements, incomplete polarizations were observed even at exactly $\nu = 1$, showing that the $\nu = 1$ condition itself cannot be used as a reliable reference. We have decided to use instead the robust $\nu = 2/3$ fractional quantum Hall state, which is known to host electron domains which can be either fully spin polarized $P = 1$ or unpolarized $P = 0$.[5,10] f-PRDNMR measurements at $\nu = 2/3$ therefore enable us to determine both the $f_0$ value, characterizing the response of unpolarized electrons, and the "maximal" value of the Knight shift $\Delta f_{2/3} = f_{2/3} - f_0$ where $f_{2/3}$ is the lower frequency response emerging from the $P = 1$ electron domains.

For each magnetic field (electron densities), $\nu = 2/3$ calibration experiments were performed in the same radio frequency conditions and using the same detection point as for $\nu \sim 1$. In each case the hyperfine coupling constant $\mathcal{A}$ satisfies the relation: $\Delta f_{2/3} = \mathcal{A} \times n_{2/3}/W$, valid for a fully polarized electron system characterized by a physical width $W$. A density dependence of the 2DEG width $W$ may play a significant role in modulating $\Delta f$ when different electron densities (widths) are involved. The measured product $(\Delta f_{2/3}/n_{2/3}) \times (n_{2/3})^{-1/3}$ was found to be constant within 3% on our entire field/density range, showing that $W$ follows a $W \propto n^{-1/3}$ law. Such a behavior can be accounted for from band structure simulations of the GaAs quantum well studied here.

To compare polarization obtained in experiments with different magnetic fields, we have chosen to use a single value of $\mathcal{A}$ average over the experimentally determined values. The spin polarization of the system at a filling factor $\nu$ is then obtained by writing : $P_\nu = (\Delta f_\nu/n_\nu) \times (W_\nu/\mathcal{A})$, which leads to $P_\nu = (\Delta f_\nu/\Delta f_{2/3}) \times (n_{2/3}/n_\nu)^{4/3}$. The resonant frequency $f_r$ defining the frequency shift $\Delta f = f_r - f_0$ was determined from the position of the $R_{xx}$ minimum, as explained in the previous paragraph. The determination of $P$ is therefore direct since $\Delta f_\nu$, $\Delta f_{2/3}$, and the electron densities are all experimentally measured.

## III. QHF VERSUS SKYRMION GLASS: EXPERIMENTAL PHASE DIAGRAM

### A. Coulomb interactions

To allow a comparison between the theoretical[11,12] and experimental phase diagrams, a realistic estimation of the Coulomb energy in our system is needed. This is particularly required due to the well-known discrepancies between the pure Coulomb energy $E_c = e^2/(4\pi\epsilon_0\epsilon_r l_B)$ and its value in non-ideal 2D systems with non-zero disorder and finite thickness along the confinement axis. Our approach to estimate experimentally the quantity $E_c$ is based on energy gap measurements at $\nu = 1$.

In the case of spin wave excitations of the quantum Hall ferromagnet,[13] and for charged excitation (infinite momentum transfer) detected in transport, the $\nu = 1$ energy gap $E_s$ is linked to the Coulomb $E_c$ energy by:

$$E_s = |g^*\mu_B B| + \sqrt{\pi/2}E_c \qquad (2)$$

where $\sqrt{\pi/2}$ is the spin stiffness constant. In the presence of Skyrmions, the excitation gap is known to be further reduced,[14,15] which is why we have decided to employ tilted-field measurements to boost the $\eta$ ratio and reduce the influence of skyrmions.

The $\nu = 1$ activation gap $\Delta_{\nu=1}$ was studied at $B_F = 6T$ for different $B_{tot}$ values (see table I). $\Delta_{\nu=1}$ was extracted as usually done in the thermally activated regime of the longitudinal resistance $R_{xx}$ where $R_{xx} \propto e^{-\Delta_{\nu=1}/2k_BT}$. The obtained $\Delta_{\nu=1}$ vs $B_{tot}$ dependance shows the usual "saturating trend" due to the reduction of the Skymions size as $B_{tot}$ (and $\eta$) increases.[14] From these data one can estimate the Skyrmion-modified Zeeman energy contribution which we found in the high $B_{tot}$ region to be about $1.6|g^*|\mu_B B$. The experimental Coulomb energy is then estimated by withdrawing this Zeeman energy contribution from $\Delta_{\nu=1}$ and taking into account the disorder broadening $\Gamma$ which differentiates activation gaps from spectral gap:

$$E_c^{exp} = \sqrt{2/\pi}(\Delta_{\nu=1} + \Gamma - 1.6|g^*|\mu_B B) \qquad (3)$$

From the experimentally determined value at $B_F = 6T$, 24.5 K, $E_c^{exp}$ is estimated at different value of $B_F$ assuming a simple $\sqrt{B}$ dependence expected for Coulomb interaction, giving $E_c^{exp} = 10.02\sqrt{B}$.

### B. Disorder

As can be seen through the mobility reported in table I, the amount of disorder in our sample may vary with the electron density, being larger as the screening is reduced at low electron densities. It is nevertheless well-known that the mobility gives a limited characterization of disorder at the quantum level in a 2DEG. To obtain a more precise description of disorder, we have measured the Landau level broadening from Shubnikov-de Haas oscillations. The measurements were performed in the limit of zero temperature (10 mK) for four different electron densities covering our entire range of work.

The data have been analyzed with the traditional Lifshitz-Kosevich formalism, using Gaussian Landau level for the electronic density of states.[16] The obtained full width at half maximum (FWHM) of Gaussian Landau levels are reported in table I. $\Gamma$ decreases slightly with increasing density, qualitatively consistent with the increase observed in the electron mobility. However, we note that the increase in $\Gamma$ is much weaker than the linear increase observed for $\mu$. This is due to the fact that the scattering in our sample is dominantly of long-range nature, and increasing the electron density essentially eliminates the minority short-range scattering processes which control the electron mobility.

| $n$ $(cm^{-2})$ | $\mu$ $(10^6 cm^2/Vs)$ | $\Gamma$ (K) | $B_F(T)$ | $B_{tot}(T)$ | $\Delta_{\nu=1}$ (K) | $E_c^{exp}(K)$ | $\gamma_{int}$ |
|---|---|---|---|---|---|---|---|
| 1.2 | 0.30 | 5.68 | 5 | 5 | - | 22.36 | 3.93 |
| 1.44 | 0.36 | 5.5 | 6 | 6 | 26.94 | 24.5 | 3.93 |
| 1.44 | 0.36 | - | 6 | 11.37 | 30.64 | 24.5 | 3.93 |
| 1.44 | 0.36 | - | 6 | 12.13 | 30.98 | 24.5 | 3.93 |
| 1.44 | 0.36 | - | 6 | 13.87 | 31.95 | 24.5 | 3.93 |
| 1.73 | 0.44 | 5.47 | 7.2 | 7.2 | | 26.84 | 4.9 |
| 1.73 | 0.44 | - | 7.2 | 14 | - | | |
| 2.17 | 0.54 | 5.31 | 9 | 9 | - | 30 | 5.65 |
| 2.65 | 0.65 | 5.16 | 11 | 11 | - | 33.17 | 6.43 |
| 3.37 | 0.84 | 4.96 | 14 | 14 | - | 37.42 | 7.54 |

TABLE I: Characteristics of the 2DEG sample: electron density $n$, low temperature mobility $\mu$, Landau level FWHM $\Gamma$, perpendicular magnetic field $B_F$ corresponding to $\nu = n/(eB/h) = 1$, total applied magnetic field $B_{tot}$, activation gap at $\nu = 1$ $\Delta_{\nu=1}$ , experimental Coulomb energy $E_c^{exp}$, ratio between experimental Coulomb energy and disorder $\gamma_{int} = E_c^{exp}/\Gamma$.


[1] S. E. Barrett, R. Tycko, L. N. Pfeiffer, and K. W. West, Phys. Rev. Lett. **72**, 1368 (1994), URL http://link.aps.org/doi/10.1103/PhysRevLett.72.1368.

[2] S. Melinte, N. Freytag, M. Horvatić, C. Berthier, L. P. Lévy, V. Bayot, and M. Shayegan, Phys. Rev. Lett. **84**, 354 (2000), URL http://link.aps.org/doi/10.1103/PhysRevLett.84.354.

[3] W. Desrat, D. K. Maude, M. Potemski, J. C. Portal, Z. R. Wasilewski, and G. Hill, Phys. Rev. Lett. **88**, 256807 (2002).

[4] L. Tiemann, G. Gamez, N. Kumada, and K. Muraki, Science **335**, 828 (2012).

[5] M. Stern, B. A. Piot, Y. Vardi, V. Umansky, P. Plochocka, D. K. Maude, and I. Bar-Joseph, Phys. Rev. Lett. **108**, 066810 (2012), URL http://link.aps.org/doi/10.1103/PhysRevLett.108.066810.

[6] R. Tycko, S. Barrett, G. Dabbagh, L. Pfeiffer, and K. West, Science **268**, 1460 (1995), http://www.sciencemag.org/content/268/5216/1460.full.pdf, URL http://www.sciencemag.org/content/268/5216/1460.abstract.

[7] W. Desrat, B. A. Piot, S. Krämer, D. K. Maude, Z. R. Wasilewski, M. Henini, and R. Airey, Phys. Rev. B **88**, 241306 (2013), URL http://link.aps.org/doi/10.1103/PhysRevB.88.241306.

[8] This is further demonstrated by the fact that the polarization of the system can be full while the maximum feature is still present in the NMR response. In this sense, the response is similar to the one observed at $\nu = 2/3$ where spatially independent domains of different spin polarization coexist.

[9] B.A. Piot, W. Desrat et al., in preparation.

[10] O. Stern, N. Freytag, A. Fay, W. Dietsche, J. H. Smet, K. von Klitzing, D. Schuh, and W. Wegscheider, Phys. Rev. B **70**, 075318 (2004).

[11] S. Rapsch, J. T. Chalker, and D. K. K. Lee, Phys. Rev. Lett. **88**, 036801 (2002), URL http://link.aps.org/doi/10.1103/PhysRevLett.88.036801.

[12] J. Sinova, A. H. MacDonald, and S. M. Girvin, Phys. Rev. B **62**, 13579 (2000), URL http://link.aps.org/doi/10.1103/PhysRevB.62.13579.

[13] C. Kallin and B. I. Halperin, Phys. Rev. B **30**, 5655 (1984), URL http://link.aps.org/doi/10.1103/PhysRevB.30.5655.

[14] A. Schmeller, J. P. Eisenstein, L. N. Pfeiffer, and K. W. West, Phys. Rev. Lett. **75**, 4290 (1995), URL http://link.aps.org/doi/10.1103/PhysRevLett.75.4290.

[15] D. K. Maude, M. Potemski, J. C. Portal, M. Henini, L. Eaves, G. Hill, and M. A. Pate, Phys. Rev. Lett. **77**, 4604 (1996), URL http://link.aps.org/doi/10.1103/PhysRevLett.77.4604.

[16] B. A. Piot, D. K. Maude, M. Henini, Z. R. Wasilewski, K. J. Friedland, R. Hey, K. H. Ploog, A. I. Toropov, R. Airey, and G. Hill, Phys. Rev. B **72**, 245325 (2005), URL http://link.aps.org/doi/10.1103/PhysRevB.72.245325.
